# Supplementary material for: Exploiting hidden structures in non-convex games for convergence to Nash equilibrium
Source: arXiv:2312.16609 source file (2023-12-27)
Supplement: Supplementary file 1 [file App-Errata.tex]

%----------------------------------------------------------------------
%%% APP: TEST
%----------------------------------------------------------------------
% !TEX root = ../Main.tex

When preparing the appendix of our paper, we noticed a number of typographic errors and omissions in our submission that could possibly cause confusion.
We clarify these minor issues below:

\begin{itemize}

    \item
    L115-116: ``smooth'' should read ``Lipschitz smooth''.
    
    \item 
    L202: The order of the summations $\sum_{\istate = 1}^{\nStates_\play}$ and $\sum_{\ilstatealt = 1}^{\nLatentStates_\play}$ in \eqref{lem:PHGFLyapunov} should be exchanged. \eqref{lem:PHGFLyapunov} should read $\dot \lyap(\state; \sol[\lstate]) = - \sum_{\play = 1}^{\nPlayers} \sum_{\ilstate = 1}^{\nLatentStates_\play} \sum_{\istate = 1}^{\nStates_\play} \parens{\lstate_{\play\ilstate} - \sol[\lstate_{\play\ilstate}]} \frac{\pd \lstate_{\play\ilstate}}{\pd \state_{\play\istate}} \sum_{\ilstatealt = 1}^{\nLatentStates_\play} \sum_{\istatealt = 1}^{\nStates_\play} \premat_{\play\istate\istatealt}(\state_\play)  \frac{\pd \lstate_{\play\ilstatealt}}{\pd \state_{\play\istatealt}} \frac{\pd \mloss_\play(\lstate)}{\pd \lstate_{\play\ilstatealt}}$, instead.
    
    \item
    L229: The last part of the line should read $\norm{\exof{\grad \sampled{\stochLoss_\play}{\state}}}^2 \leq \exof{\norm{\grad \sampled{\stochLoss_\play}{\state}}^2}$.
    
    \item
    L239: $\sample$ should read $\curr[\sample]$
    
    \item
    L291: The last part of the line should read ``the ergodic average $\bar\state_{\run} \in \latemap^{-1}\parens[\big]{\run^{-1} \sum_{\runalt=\start}^{\run} \lstate_{\runalt}}$''
    
    \item
    L292: Our analysis actually provides a bound for the standard restricted merit function $\gap(\ctest) = \sup_{\state\in\states} \braket{\vecfield(\latemap(\state))}{\latemap(\ctest) - \latemap(\state)}$.
    The merit function in \eqref{eq:rate-monotone} should thus read $\gap$, not $\gap_\states$.
    
    \item 
    L318: The pseudo-inverse of the Jacobian in \eqref{eq:CovariantPreconditioning} should be just simply Jacobian.
    \eqref{eq:CovariantPreconditioning} should read $\braket[\big]{\premat_\play(\state_\play) \jac[\state_\play]^\T \cvec}{\grad_{\state_\play} \lyap(\state; \lstatealt)} = \braket{\cvec}{\lstate_\play - \lstatealt_\play}.$, instead.
    
    \item 
    L322-L323: All instances of $\state$ should read $\lstate$, and $\sample$ should read $\curr[\sample]$. Specifically, \eqref{eq:PHGDEnergyBound} should read:
    $$
        \next[\lyap]
            \le \curr[\lyap] - \curr[\step] \braket[\big]{
                \vecfield(\curr[\lstate]) }{\curr[\lstate] - \lstatealt} + \curr[\step] \curr[\rand] + \curr[\step]^2 \curr[\randalt],
    $$
    where $\curr[\lyap] \defeq \lyap(\curr[\state]; \lstatealt)$, $\curr[\rand] \defeq \sum_{\play = 1}^{\nPlayers}\braket[\big]{\jac[{\curr[\state][\play]}]^\T \grad_{\curr[\lstate][\play]}(\mloss_\play(\curr[\lstate]; \curr[\sample]) - {{\mloss_\play}(\curr[\lstate])})}{\curr[\lstate][\play] - \lstatealt_\play}$, and $\curr[\randalt] \defeq \frac{\bound_1 \bound_2}{2} \norm{\curr[\est\gvec]}^2$ for some constants $\bound_1, \bound_2 > 0$.
% \item $\omega$ vs $\omega_{i,t}$
% \item The second moment of the oracle $||L(\theta,\omega)||<M^2$ instead of $\sigma^2$ in the main text
% \item Corrected typos in Lemma 6 Descent Inequality.
\end{itemize}
